# Supplementary material for: The proton charge radius extracted from the Initial State Radiation experiment at MAMI
Source: arXiv:1905.11182 source file (2019-05-27)
Supplement: Supplementary file 1 [file ISRSupplement.pdf]

# Extraction of the proton charge radius from the Initial state radiation experiment at MAMI - Supplementary material

M. Mihovilovič[a,b,c], P. Achenbach[c], T. Beranek[c], J. Beričič[b], J. C. Bernauer[d], R. Böhm[c], D. Bosnar[e], M. Cardinali[c], L. Correa[f], L. Debenjak[b], A. Denig[c], M. O. Distler[c], A. Esser[c], M. I. Ferretti Bondy[c], H. Fonvieille[f], J. M. Friedrich[g], I. Friščić[d], K. Griffioen[h], M. Hoek[c], S. Kegel[c], Y. Kohl[c], H. Merkel[c,*], D. G. Middleton[c], U. Müller[c], J. Pochodzalla[c], B. S. Schlimme[c], M. Schoth[c], F. Schulz[c], C. Sfienti[c], S. Širca[a,b], S. Štajner[b], M. Thiel[c], A. Tyukin[c], M. Vanderhaeghen[c], A. B. Weber[c]

[a] *Faculty of Mathematics and Physics, University of Ljubljana, SI-1000 Ljubljana, Slovenia*
[b] *Jožef Stefan Institute, SI-1000 Ljubljana, Slovenia*
[c] *Institut für Kernphysik, Johannes Gutenberg-Universität Mainz, DE-55128 Mainz, Germany*
[d] *Massachusetts Institute of Technology, Cambridge, MA 02139, USA*
[e] *Department of Physics, University of Zagreb, HR-10002 Zagreb, Croatia*
[f] *Université Clermont Auvergne, CNRS/IN2P3, LPC, BP 10448, F-63000 Clermont-Ferrand, France*
[g] *Technische Universität München, Physik Department, 85748 Garching, Germany*
[h] *College of William and Mary, Williamsburg, VA 23187, USA*

Table 1 collects the proton charge form factors determined by the Initial state radiation experiment for $0.001 \le Q^2 \le 0.017\,\mathrm{GeV}^2/c^2$. The new experimental results were obtained by studying the reaction H(e, e′)pγ and comparing the shape of the measured radiative tail with the simulation, using the approach explained in Ref. [1]. The extracted values, presented in the third and fourth column, were compared to the polynomial function

$$G(Q^2) = 1 - \frac{r_p^2\, Q^2}{6\,\hbar^2} + \frac{a\, Q^4}{120\,\hbar^4} - \frac{b\, Q^6}{5040\,\hbar^6}\,, \qquad (1)$$

where the parameters $a = (2.59 \pm 0.194)\,\mathrm{fm}^4$ and $b = (29.8 \pm 14.71)\,\mathrm{fm}^6$, which determine the curvature of the fit, were taken from Ref. [2]. The three data sets were fit with a common parameter for the radius, $r_p$, but with different renormalisation factors, $n_{E_0}$, for each energy, disregarding the original normalisations of the data, determined from the analysis of cross-sections. In terms of this fit with 21 degrees of freedom and $\chi^2$ of 95.4, the normalisations and the radius were determined to be:

$$\begin{aligned}
n_{195} &= 1.002 \pm 0.002_{\mathrm{stat}} \pm 0.007_{\mathrm{syst}}\,,\\
n_{330} &= 1.000 \pm 0.001_{\mathrm{stat}} \pm 0.003_{\mathrm{syst}}\,,\\
n_{495} &= 0.999 \pm 0.001_{\mathrm{stat}} \pm 0.004_{\mathrm{syst}}\,,\\
r_p &= (0.836 \pm 0.017_{\mathrm{stat}} \pm 0.059_{\mathrm{syst}} \pm 0.003_{\mathrm{mod}})\,\mathrm{fm}\,.
\end{aligned}$$

The obtained normalisation parameters were applied to renormalise the experimentally determined form factors in order to match the values of the three energy settings and to ensure consistency of the results with the statical limit $G_E^p(0) = 1$. The corrected values of $G_E^p$ with the corresponding statistical uncertainty are model dependent and are gathered in the fifth and sixth column of the table. They are also presented in Fig. 1.

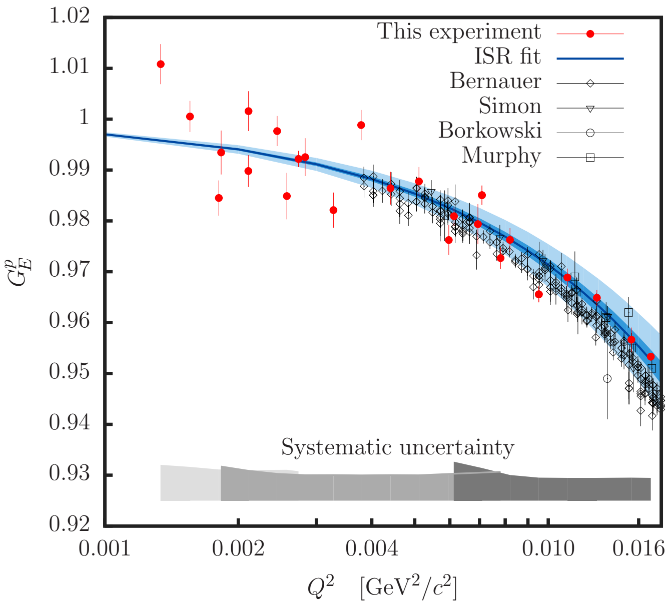


Figure 1: (Color online) The proton electric form factor as a function of $Q^2$. Empty black points show previous data [3–6]. The results of this experiment are shown with full red circles. The error bars show statistical uncertainties. Grey structures at the bottom shows the systematic uncertainties for the three energy settings. The curve corresponds to a polynomial fit to the data defined by Eq. (1). The inner and the outer bands around the fit show its uncertainties, caused by the statistical and systematic uncertainties of the data, respectively. See Ref. [1] for more details.

## References

[1] M. Mihovilovič, et al., First measurement of proton's charge form factor at very low $Q^2$ with initial state radiation, Phys. Lett. B 771 (2017) 194–198. arXiv:1612.06707, doi:10.1016/j.physletb.2017.05.031.

[2] M. O. Distler, J. C. Bernauer, T. Walcher, The {RMS} charge radius of the proton and zemach moments, Phys. Lett. B 696 (2011) 343–347. doi:http://dx.doi.org/10.1016/j.physletb.2010.12.067.

[3] J. C. Bernauer, et al., High-precision determination of the electric and magnetic form factors of the proton, Phys. Rev. Lett. 105 (2010) 242001. doi:10.1103/PhysRevLett.105.242001.

[4] G. Simon, C. Schmitt, F. Borkowski, V. Walther, Absolute electron-proton cross sections at low momentum transfer measured with a high pressure

*Corresponding author
*Email address:* merkel@kph.uni-mainz.de (H. Merkel)

Table 1: The proton charge form factors obtained with the ISR experiment at three beam energies. Results are shown as a function of $Q^2$. Third and fourth column contain directly extracted values of $G_E^p$ with the corresponding statistical uncertainties. Fifth and sixth column present renormalised values of $G_E^p$ and matching statistical uncertainties. These corrected values agree best with the quadratic function (1) and are model dependent [1]. The systematical uncertainties are divided into two parts: column seven represents the uncorrelated (point-wise) parts of the uncertainties, which influence individual measurements independently; column eight contains the correlated parts of the systematic errors, which simultaneously shifts groups of points in the same direction.

| Beam Energy [GeV] | $Q^2$ [GeV$^2/c^2$] | $G_E^p$ | Statistical uncertainty | $G_E^p$ (renormalized) | Statistical uncertainty (renormalized) | Systematical uncertainty (uncorrelated) | Systematical uncertainty (correlated) |
|---|---|---|---|---|---|---|---|
| 0.495 | 0.01704 | 0.9509 | 0.0008 | 0.9533 | 0.0008 | 0.0041 | 0.0018 |
| | 0.01540 | 0.9543 | 0.0024 | 0.9566 | 0.0024 | 0.0040 | 0.0021 |
| | 0.01288 | 0.9625 | 0.0016 | 0.9649 | 0.0016 | 0.0038 | 0.0023 |
| | 0.01105 | 0.9664 | 0.0018 | 0.9689 | 0.0018 | 0.0036 | 0.0027 |
| | 0.00952 | 0.9631 | 0.0016 | 0.9656 | 0.0016 | 0.0034 | 0.0030 |
| | 0.00820 | 0.9738 | 0.0023 | 0.9763 | 0.0023 | 0.0034 | 0.0038 |
| | 0.00709 | 0.9826 | 0.0019 | 0.9851 | 0.0019 | 0.0036 | 0.0054 |
| | 0.00613 | 0.9785 | 0.0019 | 0.9809 | 0.0019 | 0.0036 | 0.0068 |
| 0.330 | 0.00782 | 0.9726 | 0.0021 | 0.9727 | 0.0021 | 0.0048 | 0.0031 |
| | 0.00694 | 0.9793 | 0.0040 | 0.9794 | 0.0040 | 0.0046 | 0.0029 |
| | 0.00597 | 0.9762 | 0.0029 | 0.9762 | 0.0029 | 0.0044 | 0.0028 |
| | 0.00511 | 0.9877 | 0.0028 | 0.9878 | 0.0028 | 0.0043 | 0.0026 |
| | 0.00441 | 0.9864 | 0.0032 | 0.9864 | 0.0032 | 0.0044 | 0.0024 |
| | 0.00379 | 0.9988 | 0.0030 | 0.9988 | 0.0030 | 0.0044 | 0.0023 |
| | 0.00328 | 0.9820 | 0.0035 | 0.9821 | 0.0035 | 0.0045 | 0.0022 |
| | 0.00283 | 0.9925 | 0.0037 | 0.9925 | 0.0037 | 0.0046 | 0.0022 |
| | 0.00245 | 0.9976 | 0.0030 | 0.9977 | 0.0030 | 0.0049 | 0.0021 |
| | 0.00211 | 1.0015 | 0.0039 | 1.0016 | 0.0039 | 0.0055 | 0.0022 |
| | 0.00183 | 0.9933 | 0.0043 | 0.9935 | 0.0043 | 0.0063 | 0.0023 |
| 0.195 | 0.00273 | 0.9928 | 0.0016 | 0.9922 | 0.0016 | 0.0051 | 0.0028 |
| | 0.00257 | 0.9855 | 0.0046 | 0.9849 | 0.0046 | 0.0054 | 0.0028 |
| | 0.00211 | 0.9904 | 0.0031 | 0.9898 | 0.0031 | 0.0055 | 0.0025 |
| | 0.00181 | 0.9851 | 0.0035 | 0.9845 | 0.0035 | 0.0057 | 0.0024 |
| | 0.00156 | 1.0012 | 0.0031 | 1.0005 | 0.0031 | 0.0063 | 0.0023 |
| | 0.00134 | 1.0115 | 0.0039 | 1.0108 | 0.0039 | 0.0067 | 0.0021 |

gas target system, Nucl. Phys. A 333 (1980) 381–391. doi:http://dx.doi.org/10.1016/0375-9474(80)90104-9.

[5] J. J. Murphy, Y. M. Shin, D. M. Skopik, Proton form factor from 0.15 to 0.79 fm$^{-2}$, Phys. Rev. C 9 (1974) 2125–2129. doi:10.1103/PhysRevC.9.2125.
URL https://link.aps.org/doi/10.1103/PhysRevC.9.2125

[6] F. Borkowski, P. Peuser, G. Simon, V. Walther, R. Wendling, Electromagnetic form factors of the proton at low four-momentum transfer, Nucl. Phys. A 222 (1974) 269–275. doi:http://dx.doi.org/10.1016/0375-9474(74)90392-3.
